# Supplementary material for: CHORUS: Designing Human-AI Multi-Agent Collaboration for Professional Translators
Source: arXiv:2602.19016 source file (2026-09-18)
Supplement: Supplementary file 1 [file appendix.tex]

% ============================================================
% Appendix (added 2026-07-20). Content is grounded in the
% released CHORUS code (CHORUS-OSS) and the formative-study
% session transcripts. Comments starting with "AUTHORS:" mark
% items that need author verification before compiling the
% camera-ready; see appendix_verification_notes.md in the repo
% root for the evidence behind each. Delete all comments before
% uploading source to TAPS.
% ============================================================

\section{Formative Study Interview Protocol}
\label{app:interview-protocol}

The formative interviews were semi-structured and conducted in Mandarin Chinese with English code-switching. The guide below consolidates the questions used across sessions: question order and wording varied with the flow of each conversation, follow-up probes were adapted to each participant, and client-side and vendor-side experts received role-specific variants.
% AUTHORS: this guide was consolidated from the recorded session
% transcripts because no written interview guide exists in the
% project records. Please verify it against your memory of the
% sessions, and delete or add questions as appropriate.

\subsection{Part 1: Background, Workflow, and Tool Usage}
\begin{enumerate}
    \item Please describe your role: client side or vendor side, your main translation domains, and your years of professional experience.
    \item Walk me through a typical translation or post-editing task, from receiving the assignment to delivery: the steps, the tools used at each step, and the delivery standards.
    \item What materials are provided for a task (style guide, translation memory, glossaries, reference files)?
    \item How do you use AI tools in this workflow: do you use them to translate or to proofread, and what instructions or requirements do you give them?
    \item What do current AI tools do well for you, and where do they fall short? When an output feels wrong, which aspects do you find yourself checking?
    \item Which phase of the workflow is the most time-consuming or most cognitively demanding, and at which step do errors most often slip through?
    \item How do you decide that a translation is finished? What separates an acceptable deliverable from an excellent one?
    \item Do you work under deadlines, and how do you trade off efficiency against quality?
    \item How do you make sure terminology is correct, and which tools help you do so?
    \item After delivery, does anyone review your translations? When do you need to explain or justify your decisions to project managers or clients, and how are disagreements resolved?
    \item Are you familiar with MQM? Could you describe it in your own words? (The interviewer then introduced the seven dimensions used in this paper.)
    \item Which quality dimension is most problematic in current AI translations, and why? Do you check the dimensions simultaneously or in a priority order, and what signals make you prioritize one dimension over another?
    \item (Client-side experts) How is language quality assurance run on your side: which evaluation metrics are used, what happens when a delivery fails LQA, and what feedback goes back to vendors?
\end{enumerate}

\subsection{Part 2: Think-Aloud Translation Task and System Walkthrough}
Participants were then asked to translate a single English government-policy sentence in real time, starting from a deliberately awkward machine-translated Chinese draft, under the high-level instruction ``make it more formal and policy compliant.'' A low-fidelity walkthrough then illustrated how the translator's high-level goal, combined with style-guide and translation-memory context, would select the three most relevant MQM dimensions and produce three dimension-annotated candidate revisions that the translator could accept, partially adopt, or reject. Participants were asked to react to each step while thinking aloud.

\subsection{Part 3: Open-Ended Design Reflection}
\begin{enumerate}
    \item Would a system that automatically selects the most relevant MQM dimensions from your high-level instruction be useful and reliable? Besides the instruction itself, what should the selection be based on?
    \item Would you rather receive a corrected suggestion or an error annotation? Should the system show its reasoning and cite its evidence (source text, style-guide clauses, translation-memory entries), and should explanations be shown by default?
    \item If none of the candidates is satisfactory, what should happen next? How should regeneration work, how many refinement iterations would you tolerate, and what should the system do when a candidate is only partially satisfactory?
    \item How would you prefer to consume the candidates: pick the best one, splice parts of several, or keep some spans and have the rest rewritten?
    \item After the translation is finished, would an MQM-based final review that annotates remaining issues be useful? Should it report only critical errors or rank all issues by severity, and how should the annotations be displayed?
    \item What support would you want before, during, and after translating, and what would such a system have to do to earn your trust?
    \item Would this fit into your current workflow, and what would you change about the design or the interaction?
\end{enumerate}

\section{Implementation Details}
\label{app:implementation}

CHORUS is a React/TypeScript single-page application (built with Vite) backed by a single-file Flask service and a file-based memory store holding one append-only JSONL event log per user and per quality dimension. Unless stated otherwise, all LLM calls use \texttt{gpt-5.3-chat-latest} through the OpenAI API with a 2{,}048-token output cap, no sampling-temperature override, a 30-second timeout, and a single attempt backed by deterministic fallbacks; Live Style Guide reflection uses \texttt{gpt-4o-mini} with an 8-second timeout, and voice input is transcribed with \texttt{gpt-4o-mini-transcribe}. The full system, including every prompt file, is available at \url{https://github.com/iamgeorge/CHORUS-OSS}.

\subsection{Agent Prompt Templates}
\label{app:prompts}

Each of the seven agents is a static prompt file served by its own HTTP endpoint. The files share one structure, with dimension-specific content adapted from MAATS~\cite{wang2025maats}, the MQM error typology~\cite{mqm_website,lommel2018metrics}, and Unbabel's \textit{Annotation Guidelines: Typology~3.0}~\cite{unbabel_typology3}: (1) a role line restricting the agent to one dimension; (2) a scope section listing the MQM error types the agent may fix; (3) an input contract; (4) rules for using effort-weighted memory; (5) a decision policy (respect the translator's intent, make minimal edits, return the draft unchanged if it is already acceptable); and (6) a strict JSON output contract. The Accuracy agent's prompt, abridged:

\begin{footnotesize}
\begin{verbatim}
You are the **Accuracy Agent** in CHORUS.
Your only job is to improve semantic fidelity
between Source Text and Current Draft.

## Scope (Accuracy only)
Detect and fix: Addition; Omission; Mistranslation;
Hallucination; Overtranslation; Untranslated source
fragments; Wrong named entities; Completeness;
Unjustified euphemism.  [MQM taxonomy items 2.1-2.10]

## How to use memory in this new system
1. Treat higher `priority` as stronger evidence of
   user preference.
2. `live_effort` is diagnostic:
   high (>=35): user likely cared; prefer these.
   low (<20): weak/noisy; do not overfit.
3. On conflict prefer higher priority, then higher
   live_effort, then more recent examples.
4. Apply memory only when relevant to the current
   Source/Draft/Intent.
5. Never violate source meaning to satisfy style.

## Decision policy
1. Respect Translator Intent unless it would create
   an accuracy error.
2. Produce the minimal changes needed.
3. If the draft is already accurate, return it
   unchanged.

## Output (strict JSON only)
{ "revised_translation": "...",
  "explanation": "...",
  "tm_reference": "Yes/No (+ memory cited)" }
\end{verbatim}
\end{footnotesize}

\noindent At request time the backend appends the runtime inputs to the static prompt:

\begin{footnotesize}
\begin{verbatim}
### Input
Source Text:        {source_text}
Current Draft:      {current_draft}
Translator Intent:  {translator_intent}
Translation Memory (TM): {tm_context}
### Output
Return JSON only.
\end{verbatim}
\end{footnotesize}

\noindent The Fluency agent's prompt file is titled ``linguistic conventions,'' following MQM's name for that dimension; the paper and interface use \emph{Fluency} throughout. In the \textbf{Baseline} condition, the same backend serves a conventional chat assistant whose system prompt injects the source text, the initial machine-translated draft, and the translator's current draft, with no dimension decomposition, no JSON contract, and no effort-weighted memory. The complete prompt templates for all seven agents --- along with the dimension-router, stress-inference, style-guide reflection, and baseline-chat prompts --- are included in the released repository.

\subsection{Agent Ranking}
\label{app:ranking}

On each generation round all seven agents run in parallel, and their cards are ordered by
\begin{equation*}
\mathrm{score}_i \;=\; r_i^{(0)} + n_i,
\end{equation*}
where the initial relevance $r_i^{(0)} \in [0,100]$ is produced by a concurrent dimension-router LLM call that scores all seven agents against the translator's high-level goal and current editing context (naming the top three), and $n_i$ counts the translator's subsequent interactions with agent $i$ (applying a whole suggestion or a single token, regenerating, or sending the agent a follow-up request), each of which increments the score by one. Scores are not decayed; interaction counts reset when a new segment loads, and $r_i^{(0)}$ is refreshed on each generation round. The three highest-scoring agents are foregrounded and an \textit{Expand} control reveals the rest. If no router call has succeeded yet for the segment, ordering falls back to a token-level diff-magnitude heuristic, which otherwise only breaks ties.

\subsection{Live Effort Scoring}
\label{app:effort}

The frontend captures 13 behavioral signals per segment (elapsed time, initial/final pauses, edit duration, keystrokes, deletions, cursor movements, mouse selections, long pauses of ${\geq}2.5$\,s, same-region revisions, edit reversals, backward caret jumps of ${>}8$ characters, and the inferred stress score) and posts them to the backend on a debounced keystroke stream and a 1-second tick. The Live Effort score sums three capped linear components (times in seconds):
\begin{align*}
T &= \min\bigl(45,\; 0.08\,t_{\mathrm{el}} + 1.2\,\overline{t_{\mathrm{ip}}}^{12} + 0.25\,\overline{t_{\mathrm{ed}}}^{150} + 0.9\,\overline{t_{\mathrm{fp}}}^{12} + 3.5\,n_{\mathrm{lp}}\bigr)\\
K &= \min\bigl(30,\; 0.14\,n_{\mathrm{key}} + 1.4\,n_{\mathrm{del}} + 0.55\,n_{\mathrm{cur}} + 1.0\,n_{\mathrm{sel}}\bigr)\\
C &= \min\bigl(35,\; 2.4\,n_{\mathrm{rev}} + 5.0\,n_{\mathrm{und}} + 3.5\,n_{\mathrm{jmp}} + 2.5\,n_{\mathrm{lp}}\bigr) + C_{s}\\
E &= \min\bigl(100,\; T + K + C\bigr),
\end{align*}
where $\overline{x}^{c}=\min(x,c)$, $t_{\mathrm{el}}$/$t_{\mathrm{ip}}$/$t_{\mathrm{ed}}$/$t_{\mathrm{fp}}$ are the elapsed, initial-pause, edit-duration, and final-pause times, $n_{\mathrm{lp}}$/$n_{\mathrm{key}}$/$n_{\mathrm{del}}$/$n_{\mathrm{cur}}$/$n_{\mathrm{sel}}$/$n_{\mathrm{rev}}$/$n_{\mathrm{und}}$/$n_{\mathrm{jmp}}$ count long pauses, keystrokes, deletions, cursor movements, mouse selections, revisions, reversals, and jump-backs, and $C_{s}\leq 35$ is the stress term below. Scores of $E<35$, $E<65$, and $E\geq 65$ display as low, medium, and high effort.

\textbf{Stress term.} The stress-inference LLM appraises the translator's typed intent (with the source and draft as context) along Scherer's four appraisal dimensions --- difficulty, ambiguity, risk, and controllability~\cite{scherer2014nature} --- each on $[0,100]$, and returns a combined stress score $s_{\mathrm{llm}}$. This is blended with a bilingual lexical-cue heuristic as $s = 0.75\,s_{\mathrm{llm}} + 0.25\,s_{\mathrm{heur}}$, smoothed by a per-user momentum state $m$ (exponential decay $0.985^{\Delta t}$ per second, update $m \leftarrow 0.65\,m + 0.35\,s$), and enters the cognitive component as $C_{s} = \min(35,\; 0.28\,m + 0.20\,s)$, with a floor of $10 + 0.2\,(s-70)$ when $s \geq 70$.

\subsection{Memory Records and Few-Shot Injection}
\label{app:memory}

Every confirmed edit is appended as one JSONL event to the memory bucket of the agent that produced it; edits made manually without an agent share a catch-all bucket. The record below is illustrative (values abridged; the field set is as written by the system):

\begin{footnotesize}
\begin{verbatim}
{ "event_id": "...", "ts": "2026-04-02T14:31:07Z",
  "Ops": "replace",
  "old_text":    "<pre-edit target fragment>",
  "new_text":    "<post-edit target fragment>",
  "source_text": "<aligned source fragment>",
  "user_goal":   "make it more formal",
  "agent_dim": "terminology",
  "doc_id": "news_02", "segment_id": "seg_0007",
  "direction": "...",
  "effort": {
    "signals": { <the 13 raw signals> },
    "live_effort_score": 62.4,
    "effort_level": "medium",
    "inferred_stress_score": 41.0,
    "salience_score": 71.9 },
  "salience_score": 71.9 }
\end{verbatim}
\end{footnotesize}

\noindent Each event also receives a \emph{salience} score that weights its Live Effort by stability (high-effort edits that were never reversed score higher) and by its pause and edit durations. At prompt-construction time, the events in the agent's bucket are ranked by a composite retrieval priority that combines salience, Live Effort, and lexical similarity to the current intent and source text, down-weighting low-effort events; the top-ranked events --- up to eight, or the top three as a fallback --- are injected into the prompt's Translation Memory slot, each rendered as
% AUTHORS: Section 4 currently says "the top-five micro-edits";
% the deployed default is up to eight (fallback three). Align
% the Section 4 sentence with this appendix.

\begin{footnotesize}
\begin{verbatim}
1. src='...' | edit='old' -> 'new' | goal='...'
   | live_effort=72.0 | salience=81.0 | priority=77.5
\end{verbatim}
\end{footnotesize}

\noindent preceded by an instruction to treat high-effort, high-salience edits as strong preferences and low-effort edits as noise. Fuzzy-matched translation-memory entries from the user's previously completed segments (top three) are merged into the same slot. The exact salience and retrieval-priority formulas, together with the Live Style Guide generation pipeline and all remaining implementation details, are documented in the released repository.
